# Supplementary material for: Chairs Can be Stood on: Overcoming Object Bias in Human-Object Interaction Detection
Source: arXiv:2207.02400 source file (2022-07-06)

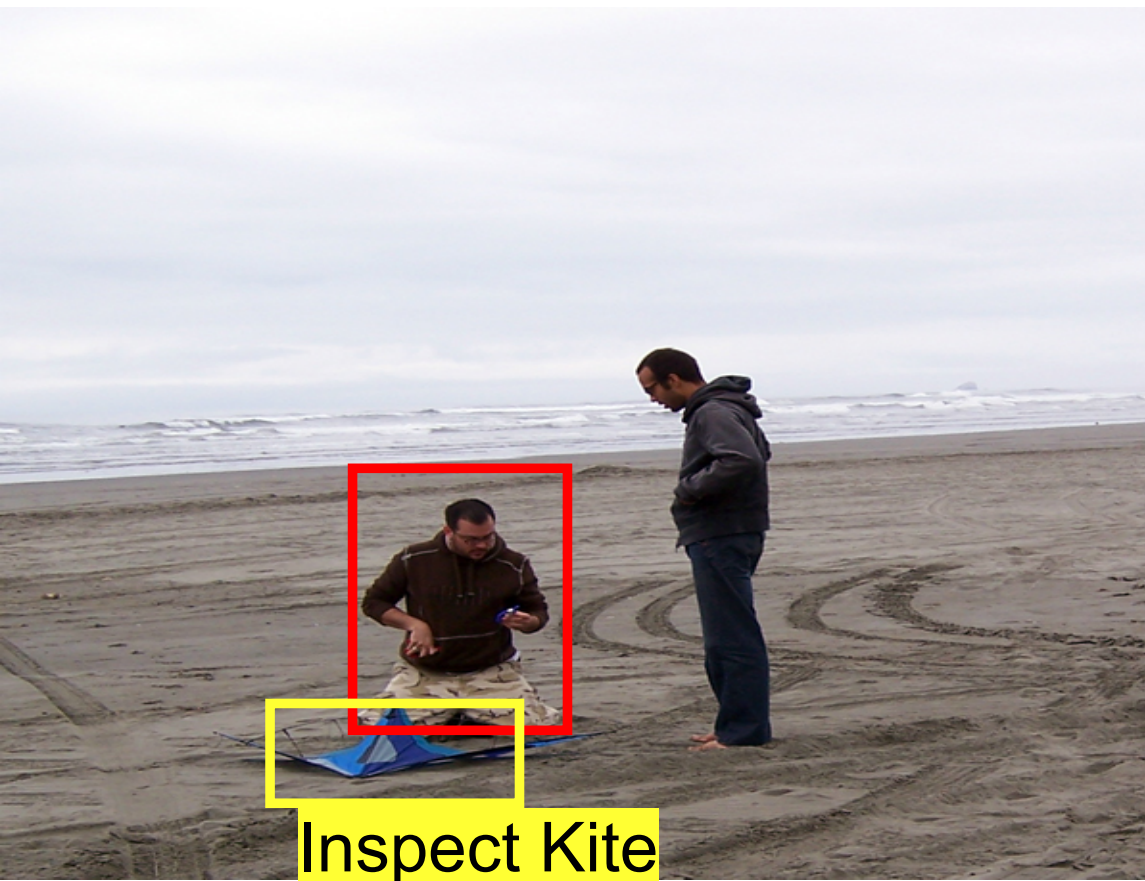

SCG: **0.024**  
Ours: **0.444**

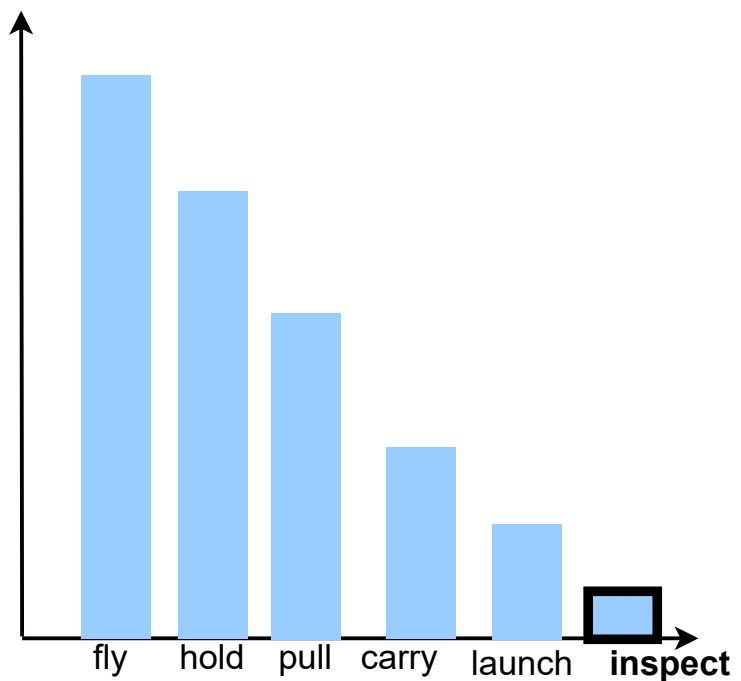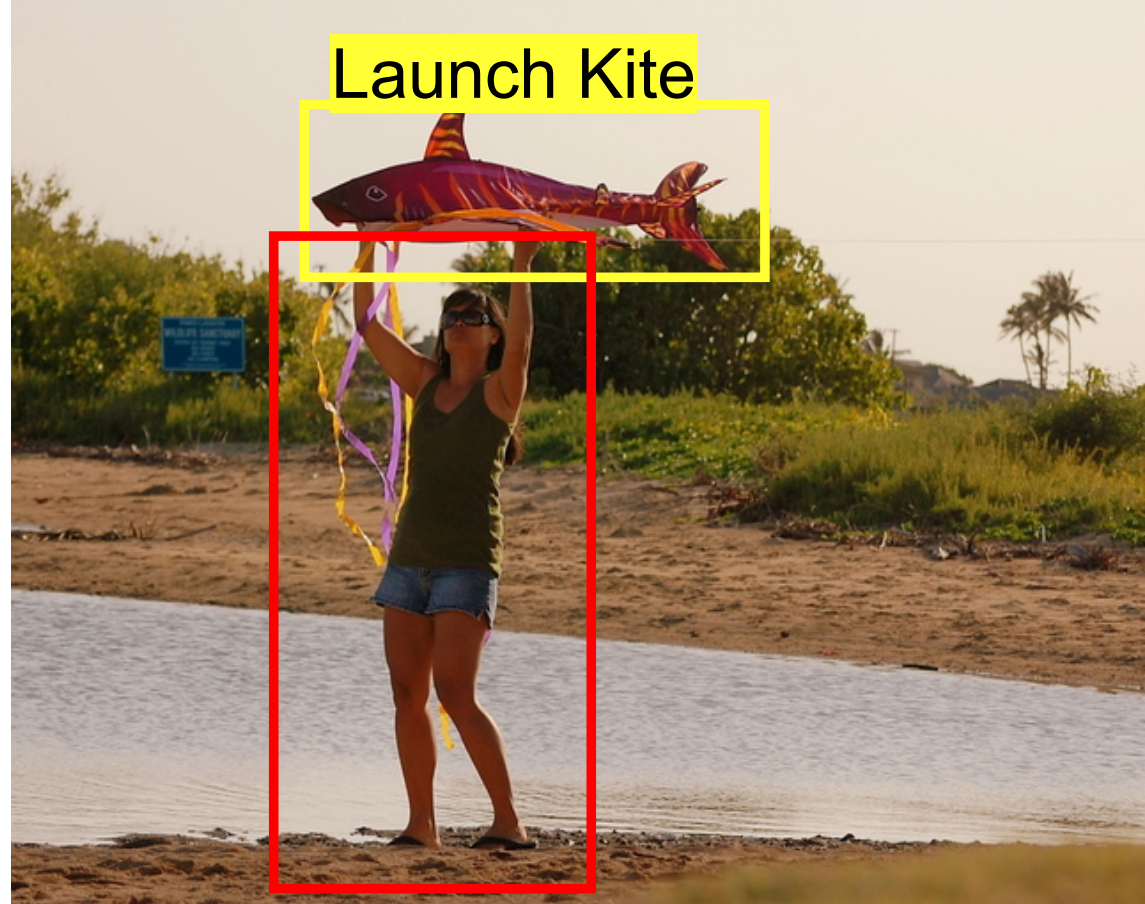

SCG: **0.032**  
Ours: **0.357**

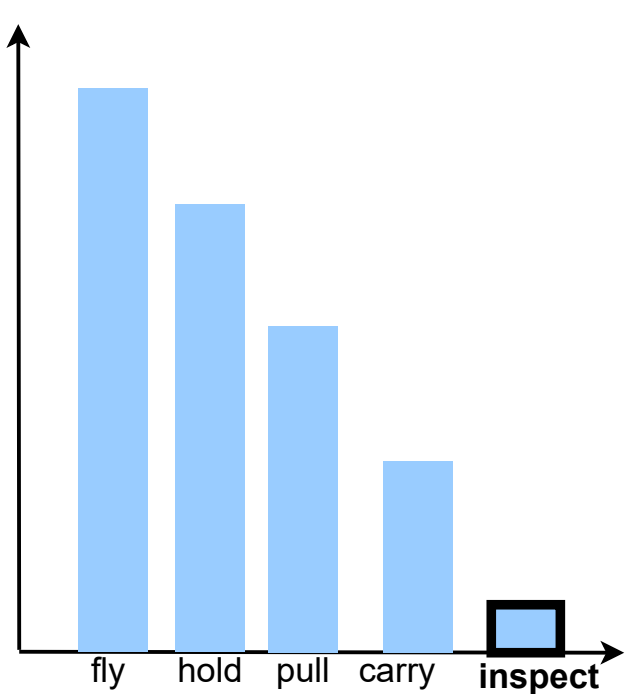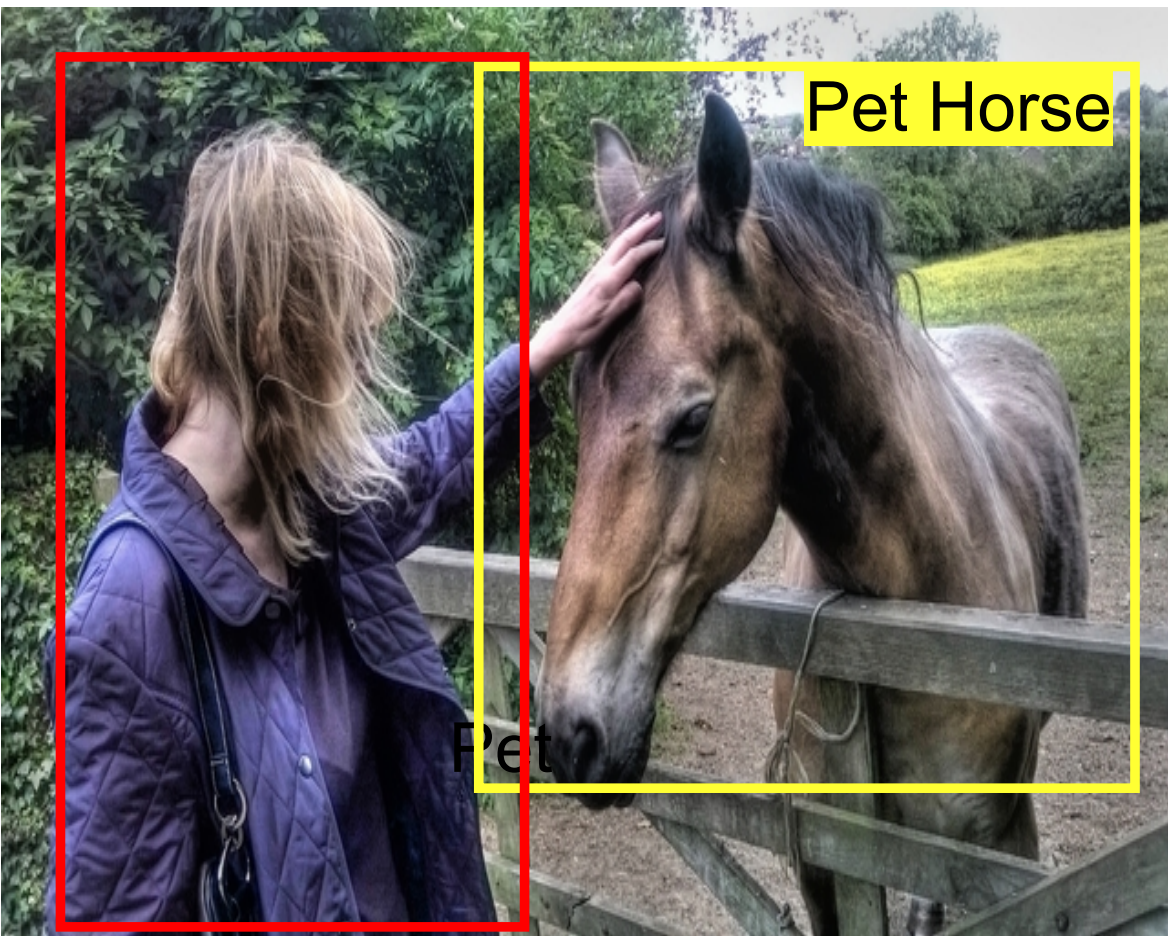

SCG: **0.208**  
Ours: **0.688**

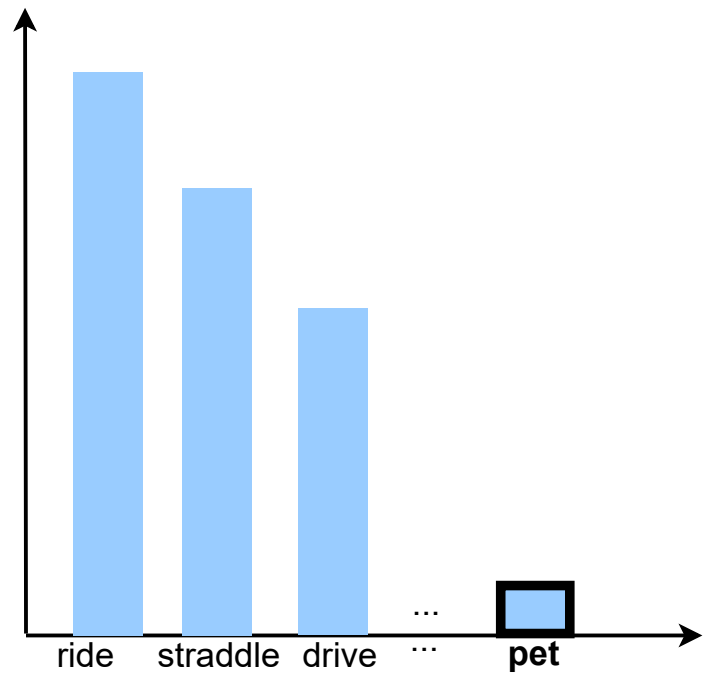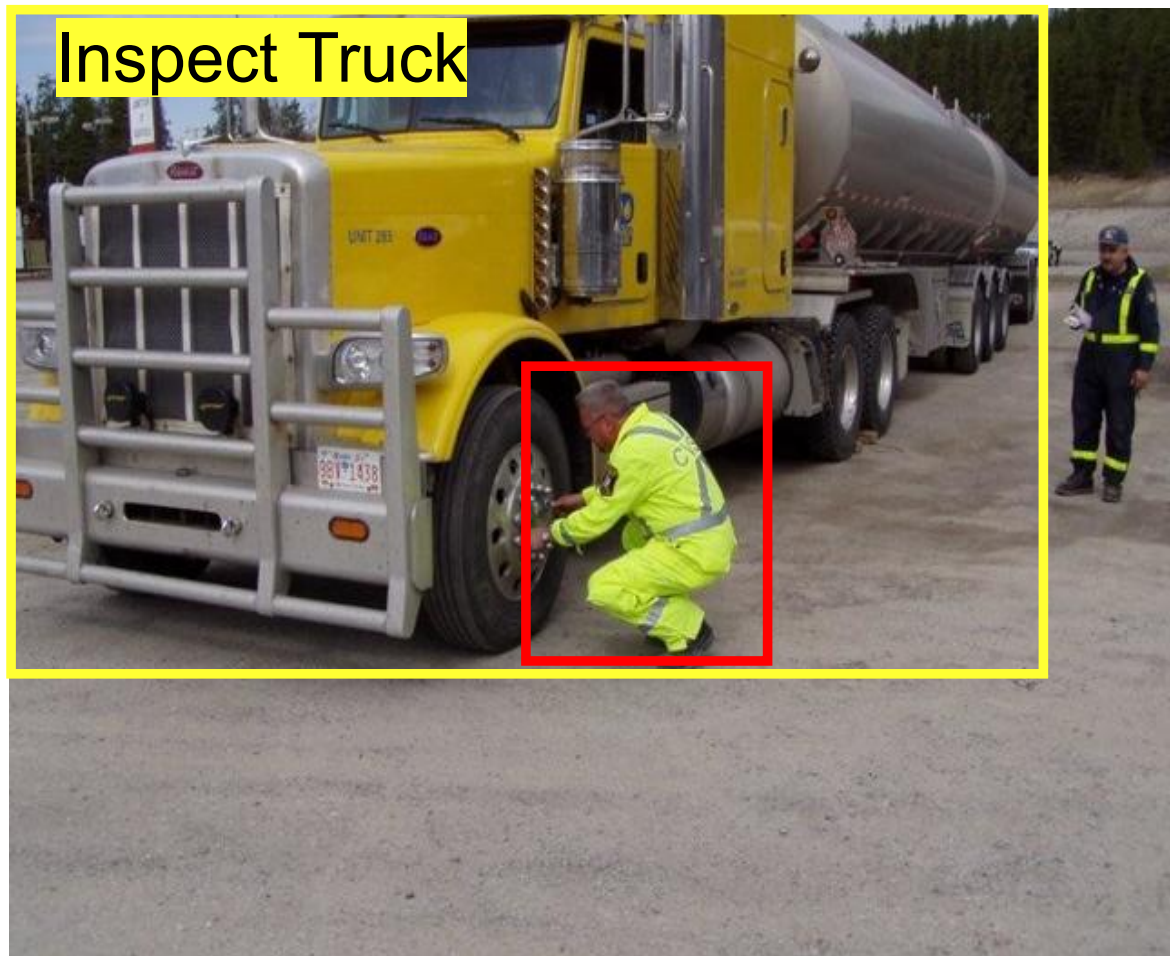

SCG: **0.014**  
Ours: **0.499**

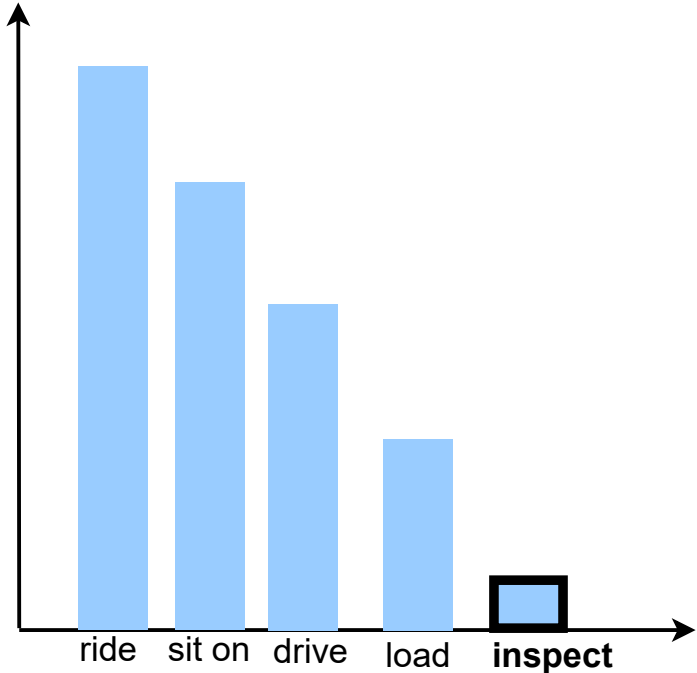

Supplement: Supplementary file 1 [file objectbias-Quali_Supp.pdf]
